# Supplementary material for: Understanding the Social Context of Eating with Multimodal Smartphone Sensing: The Role of Country Diversity
Source: arXiv:2306.00709 source file (2023-10-04)
Supplement: Supplementary file 1 [file Appendix.tex]

\appendix

\onecolumn
\newpage

\subsection*{Appendix}

% Please add the following required packages to your document preamble:
% \usepackage{booktabs}
% \usepackage{graphicx}
% \usepackage[table,xcdraw]{xcolor}
% If you use beamer only pass "xcolor=table" option, i.e. \documentclass[xcolor=table]{beamer}
\begin{table}[h]
\caption{Summary of 105 features extracted from sensing data, aggregated around activity self-reports using a time window. Detailed information can be found in \cite{generalization_across_countries}. }
\label{table_features}
\resizebox{\columnwidth}{!}{%
\begin{tabular}{@{}lll@{}}

\rowcolor[HTML]{EDEDED}
\textbf{Modality} &
  \textbf{Frequency} &
  \textbf{Corresponding features and description} \\ 

Activity &
  \begin{tabular}[c]{@{}l@{}}2 samples \\ per minute\end{tabular} &
  \begin{tabular}[c]{@{}l@{}}Derived by Google Activity Recognition API. Measures time \\ spent doing activities: still / in vehicle / on bicycle / on foot / running / tilting / \\ walking / other.\end{tabular} \\

\arrayrulecolor{Gray}
    \midrule
    
App events &
  \begin{tabular}[c]{@{}l@{}}10 samples \\ per minute\end{tabular} &
  \begin{tabular}[c]{@{}l@{}}Time spent on apps grouped by categories derived from Google Play Store: \\ action / adventure / arcade /  art \& design / auto \& vehicles /  beauty / board / \\ books \& reference / business / card / casino / casual / comics / communication /  \\ dating /  education / entertainment / finance / food \& drink / health \& fitness / house / \\ lifestyle / maps \& navigation / medical / music / news \& magazine / parenting /\\ personalization / photography / productivity / puzzle / racing / role playing / shopping / \\ simulation / social / sports / strategy / tools / travel / trivia / video players \& editors / \\ weather / word / not found\end{tabular} \\
  \arrayrulecolor{Gray}
    \midrule
    
\begin{tabular}[c]{@{}l@{}}Bluetooth \\ {[}low energy, \\ normal{]}\end{tabular} &
  \begin{tabular}[c]{@{}l@{}}1 sample \\ per minute\end{tabular} &
  \begin{tabular}[c]{@{}l@{}}Number of devices: total number of Bluetooth devices detected \\ Mean/Std/Min/Max of Received Signal Strength Indication (RSSI) : measures the \\ proximity of other existing devices.\end{tabular} \\
\arrayrulecolor{Gray}
    \midrule
\begin{tabular}[c]{@{}l@{}}Cellular {[}GSM, \\ WCDMA, LTE{]}\end{tabular} &
  \begin{tabular}[c]{@{}l@{}}1 sample \\ per minute\end{tabular} &
  \begin{tabular}[c]{@{}l@{}}Number of devices : total number of devices detected \\ Mean/Std/Min/Max of Phone signal strength\end{tabular} \\
  \arrayrulecolor{Gray}
    \midrule
Location &
  \begin{tabular}[c]{@{}l@{}}1 sample \\ per minute\end{tabular} &
  Radius of gyration, Distance traveled, Mean/Std/Min/Max Altitude \\
\arrayrulecolor{Gray}
    \midrule
Notifications &
  on change &
  \begin{tabular}[c]{@{}l@{}}Notifications posted: number of incoming notifications \\ Notifications removed: number of notifications removed by the user \\ (features calculated with and without duplicates)\end{tabular} \\
  \arrayrulecolor{Gray}
    \midrule
Proximity &
  \begin{tabular}[c]{@{}l@{}}10 samples \\ per second\end{tabular} &
  Mean/Std/Min/Max of Proximity sensor values \\
\arrayrulecolor{Gray}
    \midrule 
Screen events &
  on change &
  \begin{tabular}[c]{@{}l@{}}Number of screen episodes, Mean/Min/Max/Std of Episode Time (an episode \\ indicates the period from the time the screen turns on until it turns off)\\ Total time: total screen time during the time window\end{tabular} \\
  \arrayrulecolor{Gray}
    \midrule
    
Steps &
  \begin{tabular}[c]{@{}l@{}}10 samples \\ per second \\ or on change\end{tabular} &
  \begin{tabular}[c]{@{}l@{}}Step counter : derived using the total number of steps since the last \\ time phone turned on. \\ Steps detected: derived using event-trigger for each new step\end{tabular} \\

\arrayrulecolor{Gray}
    \midrule
Touch events &
  on change &
  Number of touch events \\

  \arrayrulecolor{Gray}
    \midrule
User presence &
  on change &
  \begin{tabular}[c]{@{}l@{}}Derived using android API, indicates the amount of time the phone was used during the \\ time window (referred as user presence).\end{tabular} \\
\arrayrulecolor{Gray}
    \midrule
    
WiFi &
  \begin{tabular}[c]{@{}l@{}}1 sample \\ per minute\end{tabular} &
  \begin{tabular}[c]{@{}l@{}}Connected to a network indicator /  Number of devices detected \\ Mean/Std/Min/Max of Received Signal Strength Indication (RSSI)\end{tabular} \\ 
  
  \arrayrulecolor{Gray}
    \bottomrule
\end{tabular}%
}
\end{table}

In this appendix, we provide detailed information about the multi-modal mobile sensing features collected by the app in the background. These features were recorded during a 10-minute window around the reported eating event, with data filtered for each sensing modality during that specific time frame.

\textbf{\textit{Activity}}: The mobile app recorded the user's activity two times per minute, based on a probability distribution of 8 activity types recognized by the Google Activity Recognition API. The API provided labels corresponding to the user's activities roughly every 30 seconds, from which we calculated a distribution of activities within seconds.

\textbf{\textit{App events}}: Due to the dataset's heterogeneity across 8 different countries, we categorized apps into app categories instead of using individual app usage. The app usage time was calculated from the time an app appeared on the screen to when it closed or went to the background. Time periods when the screen was on, but no apps were in use, were included in the "not\_found" category. Additionally, if an app couldn't fit into any category, its time period was also included in the "not\_found" category.

\textbf{\textit{Bluetooth and Wifi}}: Bluetooth features indicated whether the user was in a device-dense closed space or not. The app logged two types of Bluetooth devices: low energy and normal, along with their IDs and signal strength. Features and statistics were derived from this data. Similarly, features relative to the strength of WiFi networks in the vicinity were collected, providing indications about the user's context. Additionally, a feature indicated whether the user was connected to a network or not, which could indicate their presence in a familiar environment.

\textbf{\textit{Notifications}}: The app recorded each time a user received a notification and whether they removed it. To handle cases of duplicate notifications, we calculated the number of notifications posted by the system and removed by the user with and without duplicates.

\textbf{\textit{Location}}: Location features captured the user's movement within the time window. Data were captured once every minute using GPS or cell tower signals, resulting in a set of features.

\textbf{\textit{Proximity}}: Proximity features provided indications of the phone's location. Basic statistical features were derived from the proximity sensor readings.

\textbf{\textit{Steps}}: Two techniques were used to calculate step counts for reliability. First, the total number of steps taken since the last phone turn-on was used. Second, a separate step count called "step detected" was logged based on a trigger that sent an interrupt for every new step detected.

\textbf{\textit{Screen and touch events}}: The app logged screen on-off events with timestamps, allowing us to calculate the time users spent with their screens turned on. We also evaluated turn on-off time periods and associated them with episodes to derive statistical features. The app also logged all touch events (taps or keyboard presses), from which a feature for the total number of touch events in the time window was derived.

\iffalse
\begin{figure}[tb]
     \centering
     \includegraphics[width=0.99\linewidth]{Images/PDF/__classDist_0.pdf}
     \caption{Social Context While Eating}
     \label{dist_context}
\end{figure}

\begin{figure}[tb]
  \centering
  \includegraphics[width=\linewidth]{Images/PNG/global.png}
  \caption{Per Country Eating Report Proportions and Hourly Time Evolution of Eating Events}
  \label{time_global}
\end{figure}
\fi
